# Supplementary material for: Rethinking Nearest Neighbors for Visual Classification
Source: arXiv:2112.08459 source file (2021-12-17)
Supplement: Supplementary file 1 [file table_knnablation.tex]

\begin{table}
% \small
\scriptsize
\begin{center}
\resizebox{\columnwidth}{!}{%
\begin{tabular}{l | l  l l l }
Pooling method &max &avg &R-MAX &None \\
\hline
Accuracy (\%) & & & &
\end{tabular}
}%resize
\caption{Results on \imagenet{} using the off-the-shelf weights.}
\label{supptab:knn_pool}
\end{center}
\end{table}
